# Supplementary material for: Multi-level tree based approach for interactive graph visualization with semantic zoom
Source: arXiv:1906.05996 source file (2019-12-09)
Supplement: Supplementary file 1 [file appendix.tex]

\section*{Appendix}\label{se:Appendix}

\begin{table}[]
\parbox{.45\linewidth}{
\small
\begin{tabular}{|l|l|l|l|l|}
\hline
~&\texttt{EU}&\texttt{ST}&\texttt{NP}&\texttt{BB}&\texttt{BS}\\ \hline
\textbf{$T_1$}&1.77&15502&0.44&180830, 158202&9670\\ \hline 
\textbf{$T_2$}&2.07&123164&0.45&183078, 159150&4130\\ \hline 
\textbf{$T_3$}&2.46&479681&0.46&183391, 181196&2860\\ \hline 
\textbf{$T_4$}&2.52&851388&0.45&183391, 181196&2480\\ \hline 
\textbf{$T_5$}&2.54&1894046&0.45&183472, 181196&2100\\ \hline 
\textbf{$T_6$}&2.55&2552986&0.45&183472, 181196&1980\\ \hline 
\textbf{$T_7$}&2.58&3736676&0.46&183472, 181367&1840\\ \hline
\textbf{$T_8$}&2.60&5138014&0.46&183472, 181367&1740\\ \hline
\end{tabular}
\caption*{Direct Approach}
}
\hfill
\parbox{.45\linewidth}{
\small
% \begin{tabular}{|l|a|a|a|a|}
\begin{tabular}{|l|l|l|l|l|}
\hline
~&\texttt{EU}&\texttt{ST}&\texttt{NP}&\texttt{BB}&\texttt{BS}\\ \hline 
\textbf{$T_1$}&0.55&7185&0.37&67913, 58737&135\\ \hline 
\textbf{$T_2$}&0.71&57395&0.35&74570, 59638&631\\ \hline 
\textbf{$T_3$}&0.75&218750&0.34&74570, 61301&394\\ \hline 
\textbf{$T_4$}&0.80&382595&0.34&77507, 61327&355\\ \hline 
\textbf{$T_5$}&0.81&848433&0.34&77670, 61327&301\\ \hline 
\textbf{$T_6$}&0.83&1158137&0.34&77670, 61327&283\\ \hline 
\textbf{$T_7$}&0.83&1704918&0.34&77670, 61327&263\\ \hline 
\textbf{$T_8$}&0.84&2366331&0.34&78817, 61327&253\\ \hline
\end{tabular}
\caption*{\OurAlg}
}
\caption{Evaluation of the layout computed by Direct Approach (on the left) and \OurAlg (on the right). }
\label{tab:tabres}
\end{table}
